# Supplementary material for: Reinforcement Learning with Random Delays
Source: arXiv:2010.02966 source file (2021-05-04)
Supplement: Supplementary file 1 [file additional_calculations.tex]

% BEGIN THEOREM CDMDP  ------------------------------
\begin{theoremrep}\footnote{All theorems and lemmas are proven in the appendix.}
\label{th:cdmdp}
% old CDMDP derivation is sent in appendix as proof of this theorem
Definition \ref{def:CDMDP} defines valid MDPs in the presence of constant delays $\alpha$ and $\beta$.
\end{theoremrep}
\begin{proof}

\section{MRPs}

When both $P_{\alpha} = 0$ and $P_{\beta} = 0$, the setting is the same as in traditional RL: the observation $s_t$ is retrieved instantly, the action $a_t$ is computed instantly according to $\pi(a_t \mid s_t)$, the time-step is applied and yields the next state $s_{t+1}$ according to $p(s_{t+1} \mid s_t, a_t)$. In this setting, a Markov Reward Process (MRP) $E = (S,A,\mu,p,r)$ and a policy $\pi$ combine into a Turn-Based Markov Reward Process $\mathit{TBMRP}(E,\pi) = (S,\mu,\kappa^\pi,\overline{r}^\pi)$ such that:
$$
\kappa^\pi_{t,t+1}(s_{t+1} \mid s_{t}) = \int_{a_t \in \mathcal{A}} p(s_{t+1} \mid s_t,a_t)\pi(a_{t} \mid s_t) da_t
$$
$$
\overline{r}^\pi_{t,t+1}(s_{t}) = \int_{a_t \in \mathcal{A}} r(s_t,a_t)\pi(a_{t} \mid s_t) da_t
$$

A more advanced case has been described by \cite{ramstedt2019rtrl} under the name of Real-Time Reinforcement Learning (RTRL) setting, where $P_{\alpha} = 0$ and $P_{\beta} = 1$. In RTRL, the $1$-time-step action-delay accounts for the fact that, in real-time control, time cannot be paused during inference. The state $s_{t}$ can be augmented with the action $a_{t-1}$, whose computation ends when the state $s_{t}$ is captured, and which is to be applied until the capture of state  $s_{t+1}$. We call this augmented state $x_t=\itup{s_t,a_{t-1}} \in X$. In such case, a Markov Reward Process $E = (S,A,\mu,p,r)$ and a policy $\pi$ combine into a Real-Time Markov Reward Process $\mathit{RTMRP}(E,\pi) = (X,\mu,\kappa^\pi,\overline{r})$ such that:
$$
\kappa^\pi_{t,t+1}(\itup{s_{t+1}, a_{t}} \mid \itup{s_{t}, a_{t-1}}) = p(s_{t+1} \mid s_t,a_{t-1})\pi(a_{t} \mid \itup{s_t,a_{t-1}})
$$
$$
\overline{r}_{t,t+1}(\itup{s_{t}, a_{t-1}}) = r(s_{t}, a_{t-1})
$$
An important insight here is that, in the presence of a 1-step action-delay, the policy $\pi$ now outputs an action $a_t$ which becomes part of the next augmented state $\itup{s_{t+1}, a_t}$. As opposed to the usual turn-based setting, neither the next state $s_{t+1}$ nor the reward are affected by $a_t$ anymore. Instead, they are affected by the previous action $a_{t-1}$.

We generalize this to a fixed action-delay $P_{\beta} = \beta \geq 1$ by augmenting the state $s_t$ with a buffer of the last $\beta$ actions that have been computed. The oldest one is $a_{t-\beta}$, which is to be applied at state $s_t$ until the state $s_{t+1}$ is captured. Thus:
\begin{equation}
\kappa^\pi_{t,t+1}(\itup{s_{t+1}, \slice {\hat{a}}{t}{t-\beta+1}}  \mid  \itup{s_{t}, \slice{a}{t-1}{t-\beta}}) = p(s_{t+1} \mid s_t,a_{t-\beta})\pi(\hat{a}_{t} \mid \itup{s_{t}, \slice{a}{t-1}{t-\beta}}) \Delta_{t-\beta+1}^{t}
\end{equation}
Where $\Delta_{x}^{y} = \prod_{i=x}^{y} \delta (\hat{a}_{i} - a_i)$ is a product of Dirac densities that propagates each $a_i$ into $\hat{a}_{i}$ required so $\kappa^\pi_{t,t+1}$ is well defined as a probability distribution, and where $\slice{a}{x}{y}$ is a short-hand notation for $\{a_x, \dots, a_y\}$.

Now, back to the case where $P_{\beta} = 0$, let us consider that the observation cannot be captured instantly but that capture takes exactly one time-step, i.e. $P_{\alpha} = 1$. In this situation, we no longer have access to the current state $s_t$ to compute $a_t$, which has to be computed from the previous state $s_{t-1}$. Here, the current state $s_t$ is not observed but is described by the observed previous state $s_{t-1}$ along with the action that was applied after its capture: $a_{t-1}$. Therefore we use this pair as an augmentation of the available $s_{t-1}$ observation. The transition distribution under a given policy $\pi$ becomes:
$$
\kappa^\pi_{t,t+1}(\itup{s_{t}, a_{t}} \mid \itup{s_{t-1}, a_{t-1}}) = p(s_{t} \mid s_{t-1},a_{t-1})\pi(a_{t} \mid \itup{s_{t-1},a_{t-1}})
$$

Again, this generalizes to a fixed observation-delay $P_{\alpha} = \alpha \geq 1$ by augmenting the available observation $s_{t-\alpha}$ with a buffer of the $\alpha$ past actions that have been applied since $s_{t-\alpha}$ was captured. This yields:
\begin{equation}
\kappa^\pi_{t,t+1}(\itup{s_{t-\alpha+1}, \slice{\hat{a}}{t}{t-\alpha+1}} \mid \itup{s_{t-\alpha}, \slice{a}{t-1}{t-\alpha}}) = p(s_{t-\alpha+1} \mid s_{t-\alpha},a_{t-\alpha}) \pi(\hat{a}_{t}  \mid  \itup{s_{t-\alpha}, \slice{a}{t-1}{t-\alpha}}) \Delta^{t-1}_{t-\alpha+1}
\end{equation}

It is now easy to see how we can handle the general case of fixed positive delays $P_{\beta} = \beta \geq 1$ and $P_{\alpha} = \alpha \geq 0$ by combining these ideas, which yields the following transition distribution under policy $\pi$:
\begin{multline}
\label{eq_fixed_delays_kernel}
\kappa^\pi_{t,t+1}(\itup{s_{t-\alpha+1}, \slice{\hat{a}}{t}{t-\alpha-\beta+1}} \mid \itup{s_{t-\alpha}, \slice{a}{t-1}{t-\alpha-\beta}}) = \\ p(s_{t-\alpha+1} \mid s_{t-\alpha},a_{t-\alpha-\beta}) \pi(\hat{a}_{t}  \mid  \itup{s_{t-\alpha}, \slice{a}{t-1}{t-\alpha-\beta}}) \Delta_{t-\alpha-\beta+1}^{t-1}
\end{multline}
Here, $s_{t - \alpha}$ was captured by the remote actor and has travelled though the observation channel for $\alpha$ time-steps. The action applied at the time of its capture had previously travelled through the the action channel channel for $\beta$ time-steps, and is therefore the $(\alpha + \beta)^{th}$ (i.e the last) action present in the $\slice{a}{t-1}{t-\alpha-\beta}$ buffer: $a_{t-\alpha-\beta}$.

Note that the case where both $\alpha=0$ and $\beta=0$ is undefined as it is only compatible with the $\mathit{TBMRP}$ setting. It is reasonable to assume $\beta \geq 1$ instead, because a zero action-delay would require an instantaneous inference time, but the actual constraint is $\alpha \geq 1$ or $\beta \geq 1$.

Defining a state-reward function under policy $\pi$ is trickier when $\alpha > 0$. In practice, it is often easy to use the delayed state-reward function:
\begin{equation}
\label{eq_delayed_reward}
\overline{r}^{\mathit{delayed}}_{t,t+1} (\itup{s_{t-\alpha}, \slice{a}{t-1}{t-\alpha-\beta}}) = r(s_{t-\alpha}, a_{t-\alpha-\beta})
\end{equation}
Indeed, this function depends on the observed delayed state $s_{t-\alpha}$, and is straightforward to compute. Note however that, as we later discuss the case where $P_{\alpha}$ can output infinite delays (lost observations), this quantity will have to be ignored in such situations. However, assuming that $\alpha_t \sim P^t_{\alpha}$ and $\beta_t \sim P^t_{\beta}$ are independent and identically distributed, the expected sum of delayed rewards will still be a meaningful statistic in terms of performance.

Alternatively, we can make the assumption that, during training, the current reward is observed (e.g. by an instantaneous observer or offline for off-policy algorithms):
\begin{equation}
\label{eq_current_reward}
\overline{r}^{\mathit{instant}}_{t,t+1} (\itup{s_{t-\alpha}, \slice{a}{t-1}{t-\alpha-\beta}}) = 
\E_{s_t \sim T_p(\cdot \mid s_{t-\alpha}, \sli{a}{t-\alpha-\beta}{t-\beta-1})}[r(s_{t}, a_{t-\beta})]
\end{equation}
Where $\mathit{Tp}$ is an unrolled sub-trajectory of states defined by the delayed observation $s_{t-\alpha}$ and part of the action buffer.

Or, off-policy, we can "undelay" the rewards completely according to:
\begin{equation}
\label{eq_undelayed_reward}
\overline{r}^{\mathit{undelayed}}_{t,t+1} (\itup{s_{t-\alpha}, \slice{a}{t-1}{t-\alpha-\beta}}) = 
\E_{s_{t+\beta-1} \sim T_p(\cdot \mid s_{t-\alpha}, \sli{a}{t-\alpha-\beta}{t-2})}[r(s_{t+\beta-1}, a_{t-1})]
\end{equation}


If we want to work in the general case, we can define the reward function as:
\begin{equation}
\label{eq_fixed_delays_reward}
\overline{r}^{g}_{t,t+1}(\itup{s_{t-\alpha}, \slice{a}{t-1}{t-\alpha-\beta}}) =
\E_{s_{t-\alpha+g} \sim T_p(\cdot \mid s_{t-\alpha}, \sli{a}{t-\alpha-\beta}{t-\alpha-\beta+g-1})}[
r(s_{t-\alpha+g}, a_{t-\alpha-\beta+g})
]
\end{equation}
Where $g \in \{ 0, \dots, \alpha + \beta - 1 \}$.
The corresponding state-action reward function is:
\begin{equation}
\label{eq_fixed_delays_reward_sa}
r^{g}_{t,t+1}(\itup{s_{t-\alpha}, \slice{a}{t-1}{t-\alpha-\beta}}, a_t) =
\overline{r}^{g}_{t,t+1}(\itup{s_{t-\alpha}, \slice{a}{t-1}{t-\alpha-\beta}})
\end{equation}

Equation \ref{eq_fixed_delays_kernel} shows how a model should be built in order to handle fixed delays. Namely, the model needs an internal state in order to store the information given by the $\slice{a}{t-1}{t-\alpha-\beta}$ action buffer. Alternatively, the buffer can be fed directly to the model as part of the input space. We choose the second solution as it is easy to implement.

We can now define an adapted MRP as follows:
\begin{definition}
A Constantly Delayed Markov Reward Process $\mathit{CDMRP}(E, \pi, \alpha, \beta) = (X,\mu,\kappa^\pi,\overline{r})$ combines a Markov Decision Process $E=(S,A,\mu,p,r)$ with a policy $\pi : X \rightarrow A $, and satisfies equations \ref{eq_fixed_delays_kernel} and \ref{eq_fixed_delays_reward}.

Here, the state space is $X = S \times A^{\alpha+\beta}$, observations being $x_t = (s_{t-\alpha}, \slice{a}{t-1}{t-\alpha-\beta})$.
The initial actions can be set to a fixed value $c$, i.e. $\mu (x_0) = \mu(s_{- \alpha}) \prod_{i=-\alpha-\beta}^{-1} \delta (a_{i} - c)$.
\end{definition}


It is then possible to show that:
\begin{equation}
\mathit{CDMRP}(E, \pi, \alpha, \beta) = \mathit{TBMRP}(\mathit{CDMDP}(E, \alpha, \beta), \pi).
\end{equation}
Indeed:
$\mathit{TBMRP}(\mathit{CDMDP}(E, \alpha, \beta), \pi)$ is:

State space: $X = S \times A^{\alpha + \beta}$

Initial distribution: $\mu (x_0) = \mu(s_{- \alpha}) \prod_{i=-\alpha-\beta}^{-1} \delta (a_{i} - c)$

Transition distribution:
$$
\int_{a_t \in A} 
p(s_{t-\alpha+1} \mid s_{t-\alpha}, a_{t-\alpha-\beta}) \Delta_{t-\alpha+1-\beta}^{t} \pi(a_t \mid \itup{s_{t-\alpha}, \slice{a}{t-1}{t-\alpha-\beta}}) d a_t
$$
$$
=
p(s_{t-\alpha+1} \mid s_{t-\alpha}, a_{t-\alpha-\beta})
\Delta_{t-\alpha+1-\beta}^{t-1}
\int_{a_t \in A} 
\delta (a_t - \hat{a}_{t}) \pi(a_t \mid \itup{s_{t-\alpha}, \slice{a}{t-1}{t-\alpha-\beta}}) d a_t
$$
$$
=
p(s_{t-\alpha+1} \mid s_{t-\alpha}, a_{t-\alpha-\beta})
\pi(\hat{a}_{t} \mid \itup{s_{t-\alpha}, \slice{a}{t-1}{t-\alpha-\beta}})
\Delta_{t-\alpha+1-\beta}^{t-1}
$$

Reward function:
$$
\int_{a_t \in A} 
r^{g}_{t,t+1}(x_t, a_t)
\pi(a_t \mid \itup{s_{t-\alpha}, \slice{a}{t-1}{t-\alpha-\beta}})
d a_t
$$
$$
=
\overline{r}^{g}_{t,t+1}(x_t)
\int_{a_t \in A} 
\pi(a_t \mid \itup{s_{t-\alpha}, \slice{a}{t-1}{t-\alpha-\beta}})
d a_t
$$
$$
=
\overline{r}^{g}_{t,t+1}(x_t)
$$
Which is $\mathit{CDMRP}(E, \pi, \alpha, \beta)$.

\end{proof}
% END THEOREM CDMDP --------------------------------



Apart from vanilla SAC, we compare DC/AC to an alternative version of SAC in which we ``undelay'' the rewards off-policy, which can be done in a $\mathit{CDMDP}$ according to the following result: 

\begin{theoremrep}
Undelayed rewards have the same value as delayed rewards in a CDMDP.
In a CDMDP we can redefine rewards as
\begin{equation}
    r_\text{UD}(x_t, a_t) = \gamma^{\alpha+\beta} \E[r_\text{CDMDP}(x_{t+\alpha+\beta}, a)]
    % r_\text{UD}(\itup{s_{t-\alpha}, \slice{a}{t-1}{t-\alpha-\beta}}, a_t) = \E[]
\end{equation}
which has the same value as the original rewards.
\end{theoremrep}
\begin{proof}
...
\end{proof}
\TODO{The estimator for these undelayed rewards}





%%% APPENDIX %%%





\section{Rolled out equations}

In the constant delays setting:
\begin{equation}
v^\pi_{\mathit{CDMDP}(E, \alpha, \beta)} (x_t)
=
\mathbb{E}_{a_t \sim \pi(\cdot \mid x_t)}[
r(s_{t-\alpha}, a_{t-\alpha-\beta})
+ \mathbb{E}_{x_{t+1} \sim p(\cdot \mid x_t, a_t)}[
v^\pi_{\mathit{CDMDP}(E, \alpha, \beta)} (x_{t+1})
]
]
\end{equation}
where $x_{t} = \itup{s_{t-\alpha}, \slice{a}{t-1}{t-\alpha-\beta}}$ and $x_{t+1} = \itup{s_{t-\alpha+1}, \slice{a}{t}{t-\alpha-\beta+1}}$.


We show that the state-value can be unrolled as:
\begin{lemma}
\begin{multline}
\label{eq_cd_state_value}
v^\pi_{\mathit{CDMDP}(E, \alpha, \beta)} (\itup{s_{t-\alpha}, \slice{a}{t-1}{t-\alpha-\beta}})
=
r(s_{t-\alpha}, a_{t-\alpha-\beta}) \\
+
\mathbb{E}_{T_p}
[
\sum_{i=t-\alpha-\beta+1}^{t-1} r(s_{i + \beta}, a_{i})
+
\mathbb{E}_{T_\pi}
[
v^\pi_{\mathit{CDMDP}(E, \alpha, \beta)} (\itup{s_{t+\beta}, \slice{a}{t+\alpha+\beta-1}{t}})]]
\end{multline}

where 
%\[
$
\left\{
\begin{array}{l}
T_p: \slice s {t+\beta}{t-\alpha+1} \sim p((s_{t-\alpha},a_{t-\alpha-\beta}), \dots, (s_{t+\beta-1},a_{t-1}))\\
T_\pi: \slice a {t+\alpha+\beta-1}{t} \sim \pi(\itup{s_{t-\alpha}, \slice{a}{t-1}{t-\alpha-\beta}}, \dots, \itup{s_{t+\beta-1}, \slice{a}{t+\alpha+\beta-2}{t-1}})
\end{array}
\right.
%\]
$
\end{lemma}

\begin{proof}
\begin{multline}
v^\pi_{\mathit{CDMDP}(E, \alpha, \beta)} (\itup{s_{t-\alpha}, \slice{a}{t-1}{t-\alpha-\beta}}) \\
=
\mathbb{E}_{a_{t} \sim \pi(\cdot \mid \itup{s_{t-\alpha}, \slice{a}{t-1}{t-\alpha-\beta}})}
[ \\
r(s_{t-\alpha}, a_{t-\alpha-\beta}) \\
+
\mathbb{E}_{s_{t-\alpha+1} \sim p(\cdot \mid s_{t-\alpha}, a_{t-\alpha-\beta})}
[ \\
v^\pi_{\mathit{CDMDP}(E, \alpha, \beta)} (\itup{s_{t-\alpha+1}, \slice{a}{t}{t-\alpha-\beta+1}})]]
\end{multline}
\begin{multline}
=
r(s_{t-\alpha}, a_{t-\alpha-\beta}) \\
+
\mathbb{E}_{a_{t} \sim \pi(\cdot \mid \itup{s_{t-\alpha}, \slice{a}{t-1}{t-\alpha-\beta}})}
[ \\
\mathbb{E}_{s_{t-\alpha+1} \sim p(\cdot \mid s_{t-\alpha}, a_{t-\alpha-\beta})}
[ \\
v^\pi_{\mathit{CDMDP}(E, \alpha, \beta)} (\itup{s_{t-\alpha+1}, \slice{a}{t}{t-\alpha-\beta+1}})]]
\end{multline}
\begin{multline}
=
r(s_{t-\alpha}, a_{t-\alpha-\beta}) \\
+
\mathbb{E}_{a_{t} \sim \pi(\cdot \mid \itup{s_{t-\alpha}, \slice{a}{t-1}{t-\alpha-\beta}})}
[ \\
\mathbb{E}_{s_{t-\alpha+1} \sim p(\cdot \mid s_{t-\alpha}, a_{t-\alpha-\beta})}
[ \\
\mathbb{E}_{a_{t+1} \sim \pi(\cdot \mid \itup{s_{t-\alpha+1}, \slice{a}{t}{t-\alpha-\beta+1}})}
[ \\
r(s_{t-\alpha+1}, a_{t-\alpha-\beta+1}) \\
+
\mathbb{E}_{s_{t-\alpha+2} \sim p(\cdot \mid s_{t-\alpha+1}, a_{t-\alpha-\beta+1})}
[ \\
v^\pi_{\mathit{CDMDP}(E, \alpha, \beta)} (\itup{s_{t-\alpha+2}, \slice{a}{t+1}{t-\alpha-\beta+2}})]]
]]
\end{multline}
\begin{multline}
=
r(s_{t-\alpha}, a_{t-\alpha-\beta}) \\
+
\mathbb{E}_{s_{t-\alpha+1} \sim p(\cdot \mid s_{t-\alpha}, a_{t-\alpha-\beta})}
[ \\
r(s_{t-\alpha+1}, a_{t-\alpha-\beta+1}) \\
+
\mathbb{E}_{s_{t-\alpha+2} \sim p(\cdot \mid s_{t-\alpha+1}, a_{t-\alpha-\beta+1})}
[ \\
\mathbb{E}_{a_{t} \sim \pi(\cdot \mid \itup{s_{t-\alpha}, \slice{a}{t-1}{t-\alpha-\beta}})}
[ \\
\mathbb{E}_{a_{t+1} \sim \pi(\cdot \mid \itup{s_{t-\alpha+1}, \slice{a}{t}{t-\alpha-\beta+1}})}
[ \\
v^\pi_{\mathit{CDMDP}(E, \alpha, \beta)} (\itup{s_{t-\alpha+2}, \slice{a}{t+1}{t-\alpha-\beta+2}})]]
]]
\end{multline}

$$
= ( \dots )
$$

\begin{multline}
\Rightarrow
v^\pi_{\mathit{CDMDP}(E, \alpha, \beta)} (\itup{s_{t-\alpha}, \slice{a}{t-1}{t-\alpha-\beta}})
= \\
r(s_{t-\alpha}, a_{t-\alpha-\beta}) \\
+
\mathbb{E}_{s_{t-\alpha+1} , \dots , s_{t+\beta} \sim T_p(\dots \mid s_{t-\alpha}, \sli{a}{t-\alpha-\beta}{t-1})}
[ \\
\sum_{i=t-\alpha-\beta+1}^{t-1} r(s_{i + \beta}, a_{i}) \\
+
\mathbb{E}_{a_{t}, \dots, a_{t+\alpha+\beta-1}  \sim T_\pi(\dots \mid \itup{s_{t-\alpha}, \slice{a}{t-1}{t-\alpha-\beta}}, \dots, \itup{s_{t+\beta-1}, \slice{a}{t+\alpha+\beta-2}{t-1}})}
[ \\
v^\pi_{\mathit{CDMDP}(E, \alpha, \beta)} (\itup{s_{t+\beta}, \slice{a}{t+\alpha+\beta-1}{t}})]]
\end{multline}
\end{proof}

Note that, as previously pointed out, the augmented state $x_t = \itup{s_{t-\alpha}, \slice{a}{t-1}{t-\alpha-\beta}}$ is a statistic of $s_{t+\beta}$, and therefore of all the delayed rewards from $r(s_{t-\alpha},a_{t-\alpha-\beta})$ to $r(s_{t+\beta-1},a_{t-1})$.



\begin{lemmarep}
\label{lem:unrolled_dcac_value_target}
{\small
\begin{multline}
\medmuskip=0mu
\thinmuskip=0mu
\thickmuskip=0mu
v(\itup{s_{t-\alpha}, \slice{a}{t-1}{t-\alpha-\beta}})
=
\mathbb{E}_{T_p}[\mkern-18mu \sum_{i=t}^{t+\alpha+\beta-1} \mkern-20mu 
\gamma^{i-t}
r(s_{i-\alpha}, a_{i-\alpha-\beta})
+ \\
\mathbb{E}_{T_\pi}
[\mkern-8mu \sum_{i=t}^{t+\alpha+\beta-1} \mkern-10mu - \gamma^{i-t} \log \pi(a_i |\itup{s_{i-\alpha}, \slice a {i-1}{i-\alpha-\beta}})
+ \gamma^{\alpha+\beta} v(\itup{s_{t+\beta}, \slice a {t+\alpha+\beta-1}{t}})
]]
\end{multline}
}
where 
%\[
$
\left\{
\begin{array}{l}
T_p: \slice s {t+\beta}{t-\alpha+1} \sim p((s_{t-\alpha},a_{t-\alpha-\beta}), \dots, (s_{t+\beta-1},a_{t-1}))\\
T_\pi: \slice a {t+\alpha+\beta-1}{t} \sim \pi(\itup{s_{t-\alpha}, \slice{a}{t-1}{t-\alpha-\beta}}, \dots, \itup{s_{t+\beta-1}, \slice{a}{t+\alpha+\beta-2}{t-1}})
\end{array}
\right.
%\]
$

are trajectories unrolled from the augmented state $x_t$.
\end{lemmarep}
\begin{proof}
\begin{multline}
v (\itup{s_{t-\alpha},\slice{a}{t-1}{t-\alpha-\beta}}) =
\E_{s_{t-\alpha+1} \sim p(\cdot \mid s_{t-\alpha}, a_{t-\alpha-\beta})}[ \\
r(s_{t-\alpha}, a_{t-\alpha-\beta}) \\
+ \E_{a_{t} \sim \pi(\cdot \mid \itup{s_{t-\alpha},\slice{a}{t-1}{t-\alpha-\beta}})}[ \\
- \log \pi(a_{t} \mid \itup{s_{t-\alpha},\slice{a}{t-1}{t-\alpha-\beta}}) \\
\gamma v(\itup{s_{t-\alpha+1},\slice{a}{t}{t-\alpha-\beta+1}})]]
\end{multline}
\begin{multline}
v (\itup{s_{t-\alpha},\slice{a}{t-1}{t-\alpha-\beta}}) =
\E_{s_{t-\alpha+1} \sim p(\cdot \mid s_{t-\alpha}, a_{t-\alpha-\beta})}[ \\
r(s_{t-\alpha}, a_{t-\alpha-\beta}) \\
+ \E_{a_{t} \sim \pi(\cdot \mid \itup{s_{t-\alpha},\slice{a}{t-1}{t-\alpha-\beta}})}[ \\
- \log \pi(a_{t} \mid \itup{s_{t-\alpha},\slice{a}{t-1}{t-\alpha-\beta}}) \\
\gamma
\E_{s_{t-\alpha+2} \sim p(\cdot \mid s_{t-\alpha+1}, a_{t-\alpha-\beta+1})}[ \\
r(s_{t-\alpha+1}, a_{t-\alpha-\beta+1}) \\
+ \E_{a_{t+1} \sim \pi(\cdot \mid \itup{s_{t-\alpha+1},\slice{a}{t}{t-\alpha-\beta+1}})}[ \\
- \log \pi(a_{t+1} \mid \itup{s_{t-\alpha+1},\slice{a}{t}{t-\alpha-\beta+1}}) \\
\gamma v(\itup{s_{t-\alpha+2},\slice{a}{t+1}{t-\alpha-\beta+2}})]]]]
\end{multline}
\begin{multline}
v (\itup{s_{t-\alpha},\slice{a}{t-1}{t-\alpha-\beta}}) =
\E_{s_{t-\alpha+1} \sim p(\cdot \mid s_{t-\alpha}, a_{t-\alpha-\beta})}[ 
\E_{s_{t-\alpha+2} \sim p(\cdot \mid s_{t-\alpha+1}, a_{t-\alpha-\beta+1})}[ \\
r(s_{t-\alpha}, a_{t-\alpha-\beta})
+ \gamma r(s_{t-\alpha+1}, a_{t-\alpha-\beta+1}) \\
+ \E_{a_{t} \sim \pi(\cdot \mid \itup{s_{t-\alpha},\slice{a}{t-1}{t-\alpha-\beta}})}[ \E_{a_{t+1} \sim \pi(\cdot \mid \itup{s_{t-\alpha+1},\slice{a}{t}{t-\alpha-\beta+1}})}[ \\
- \log \pi(a_{t} \mid \itup{s_{t-\alpha},\slice{a}{t-1}{t-\alpha-\beta}})
- \gamma \log \pi(a_{t+1} \mid \itup{s_{t-\alpha+1},\slice{a}{t}{t-\alpha-\beta+1}}) \\
+ \gamma^2 v(\itup{s_{t-\alpha+2},\slice{a}{t+1}{t-\alpha-\beta+2}})]]]]
\end{multline}

\begin{multline}
(\dots) \\
\Rightarrow
v (\itup{s_{t-\alpha},\slice{a}{t-1}{t-\alpha-\beta}}) = \\
\E_{\sli{s}{t-\alpha+1}{t+\beta} \sim T_p(\dots \mid s_{t-\alpha}, \sli{a}{t-\alpha-\beta}{t-1})}[ \\
\sum_{i=0}^{\alpha+\beta-1}
\gamma^i r(s_{t-\alpha+i}, a_{t-\alpha-\beta+i}) \\
+ \E_{\sli{a}{t}{t+\alpha+\beta-1} \sim T_\pi(\dots \mid \itup{s_{t-\alpha},\slice{a}{t-1}{t-\alpha-\beta}}, \dots, \itup{s_{t+\beta-1},\slice{a}{t+\alpha+\beta-2}{t-1}})}[ \\
- \sum_{i=0}^{\alpha+\beta-1} \gamma^{i} \log \pi(a_{t+i} \mid \itup{s_{t-\alpha+i},\slice{a}{t-1+i}{t-\alpha-\beta+i}}) \\
+
\gamma^{\alpha+\beta} v(\itup{s_{t+\beta},\slice{a}{t+\alpha+\beta-1}{t}})
]]
\end{multline}
\end{proof}


%%% HYPERPARAMETERS %%%

%%% DEFINITIONS %%%

\section{Definitions}

\begin{definition} \label{def:TBMDP}
A Turn-Based Markov Decision Process $(Z, A, \nu, q, \rho) = T\!B\!M\!D\!P(E)$ augments another Markov Decision Process $E = (S, A, \mu, p, r)$, such that
%
\begin{flalign*}
    &\text{(1) state space} && Z = S \times \{0, 1\}, \\
    &\text{(2) action space} && A, \\
    &\text{(3) initial state distribution} && \nu(\itup{s_0, b_0}) = \mu(s_0) \ \delta(b_0), \\
    &\text{(4) transition distribution} && q(\itup{s_{t+1}, b_{t+1}} | \itup{s_t, b_t}, a_t) = \begin{cases}
            \delta(s_{t+1}-s_t) \ \delta(b_{t+1}-1) & \text{if} \ b_t = 0 \\
            p(s_{t+1} | s_t, a_t) \ \delta(b_{t+1}) & \text{if} \ b_t = 1
        \end{cases} \\
    &\text{(5) reward function} && \rho(\itup{s, b}, a) = r(s, a) \ b.
\end{flalign*}
\end{definition}
\vspace{\baselineskip}


\begin{definition} \label{def:sub-MRP}
$\augm \Omega = (Z, \nu, \augm \kappa, \augm {\bar r})$ is a sub-MRP of $\Psi = (Z, \nu, \sigma, \bar \rho)$ if its states are sub-sampled with interval $n \in \mathbb N$ and rewards are summed over each interval, i.e. for almost all $z$
\begin{equation}
    \augm\kappa(z'|z) = \kappa^n(z'|z) \quad \text{and} \quad \augm{\bar r}(z) = v_{\Psi}^n(z).
\end{equation}
% where $\kappa^n$ is the $n$-step transition function and $v_{\Omega}^n$ is the n-step value function.
\end{definition}
\vspace{\baselineskip}


\begin{definition} \label{def:MRP-reduction}
A MRP $\Omega = (S, \mu, \kappa, \bar r)$ is a reduction of $\augm \Omega = (Z, \nu, \augm\kappa, \augm{\bar r})$ if there is a state transformation $f: \augm Z \to S$ that neither affects the evolution of states nor the rewards, i.e.
% \begin{equation}
%     \mu(s) = \int_{f^{-1}(s)} \hspace{-.7cm} \nu(z) dz
%     \quad \text{and} \quad
%     \kappa(s | f(z)) = \int_{f^{-1}(s)} \hspace{-.7cm} \augm\kappa(z' | z) \ d z' \\
%     \quad \text{and} \quad
%     \bar r(f(z)) = \augm{\bar r}(z).
%     \footnote{Here, $f^{-1}(s)$ is the set of inputs for which $f(z) = s$, i.e. $\{z \in Z : f(z)=s\}$.} \\
% \end{equation}
\begin{flalign}
    & \text{(1) state space} && S = \{f(z) : z \in Z\}, & \\
    & \text{(2) initial distribution} && \mu(s) = \int_{f^{-1}(s)} \hspace{-.7cm} \nu(z) dz, & \\
    & \text{(3) transition kernel} && \kappa(s_{t+1} | s) = \int_{f^{-1}(s_{t+1})} \hspace{-.7cm} \augm\kappa(z' | z) \ d z'
        \ \ \text{for almost all} \ z \in f^{-1}(s), & \\
    & \text{(4) state-reward function} && r(s) = \augm{\bar r}(z)
        \ \ \text{for almost all} \ z \in f^{-1}(s). & 
\end{flalign}
% where $q_\Omega^t(s)$ is the state probability at time $t$.
\end{definition}
\vspace{\baselineskip}


\begin{definition} \label{def:MRP-contains}
A MRP $\Psi$ contains another MRP $\Omega$ (we write $\Omega \propto \Psi$) if $\Psi$ works at a higher frequency and has a richer state than $\Psi$ but behaves otherwise identically. More precisely,
\begin{equation}
   \Omega \propto \Psi  \iff \text{$\Omega$ is a reduction (Def.~\ref{def:MRP-reduction}) of a sub-MRP (Def.~\ref{def:sub-MRP}) of $\Psi$.}
\end{equation}
\end{definition}
\vspace{\baselineskip}


\begin{definition}
The $n$-step transition function of a MRP $\Omega = (S, \mu, \kappa, \bar r)$ is
\begin{equation}
    \kappa^n(s_{t+n} | s_t) = \int_S \kappa(s_{t+n} |s_{t+n-1}) \kappa^{n-1}(s_{t+n-1} | s_t) \ d s_{t+n-1}. \quad \text{\big | with $\kappa^1 = \kappa$}
\end{equation}
\end{definition}
\vspace{\baselineskip}


\begin{definition}
The n-step value function $v_{\Omega}^n$ of a MRP $\Omega = (S, \mu, \kappa, \bar r)$ is
\begin{equation}
    v_{\Omega}^n(s_t) = \bar r(s_t) + \int_S \kappa(s_{t+1}|s_t) v_{\Omega}^{n-1}(s_{t+1}) \ d s_{t+1}.
    \quad \text{\big | with $v_{\Omega}^1 = \bar r$}
\end{equation}
\end{definition}





\section{Definitions}

\begin{definition}
The action-value function $q_E^\pi$ for an environment $E=(S, A, \mu, p, r)$ and a policy $\pi$ is recursively defined as:
%
\begin{equation} \label{EqQ}
    q_E^\pi(s_t, a_t) = r(s_t, a_t) + \E_{s_{t+1} \sim p(\cdot | s_t, a_t)}[ \E_{a_{t+1} \sim \pi(\cdot | s_{t+1})}[ q_E^\pi(s_{t+1}, a_{t+1})]]
\end{equation}
%
\end{definition}

\begin{definition}
The state-value function $v_E^\pi$ for an environment $E=(S, A, \mu, p, r)$ and a policy $\pi$ is recursively defined as:
%
\begin{equation}
v_E^\pi(s_t) = \E_{a_t \sim \pi(\cdot | s_t)}[r(s_t, a_t) + \E_{s_{t+1} \sim p(\cdot | s_t, a_t)}[v_E^\pi(s_{t+1})]]
\end{equation}
%
\end{definition}

\begin{definition}
\label{def:MDP}
A Markov Decision Processes (MDP) is characterized by a tuple with

(1) state space $S$, \\
(2) action space $A$, \\
(3) initial state distribution $\mu: S \to \mathbb R$, \\
(4) transition distribution {$p: S \times S \times A \to \mathbb R$}, \\
(5) reward function $r: S \times A \to \mathbb R$.
\end{definition}
% This is not how you make lists in LaTeX. What is the point of numbering if you
% don't refer to the numbers? Is this definition helping the reader in any way here?





%%% Last proof %%%


Since:
\begin{multline}
v (\itup{s',(a, \bisn u1{-1})}) = \\
\E_{\epsilon_{t+1} \sim \mathcal{N}}[
q(\itup{s',(a, \bisn u1{-1})}, a_{t+1}) 
- \log \pi(a_{t+1} \mid \itup{s',(a, \bisn u1{-1})})
]
\end{multline}

The loss becomes:
%{\small
\begin{multline}
\medmuskip=0mu
\thinmuskip=0mu
\thickmuskip=0mu
L^\text{SAC}_{\mathit{CDMDP}(E)}(\pi) = 
\E_{\itup{s,u} \sim \mathcal{D}, \epsilon \sim \mathcal{N}} [\\
\log\pi(a|\itup{s,u}) \\
- r(s, \bi u{\alpha+\beta}) \\
- \gamma \E_{s' \sim \mathcal{D}}[ \\
\E_{\epsilon_{t+1} \sim \mathcal{N}}[ \\
q(\itup{s',(a, \bisn u1{-1})}, a_{t+1}) \\
- \log \pi(a_{t+1} \mid \itup{s',(a, \bisn u1{-1})})
]]
\end{multline}
%}

Which is:
%{\small
\begin{multline}
\medmuskip=0mu
\thinmuskip=0mu
\thickmuskip=0mu
L^\text{SAC}_{\mathit{CDMDP}(E)}(\pi) = 
\E_{\itup{s,u} \sim \mathcal{D}, \epsilon \sim \mathcal{N}} [\\
\log\pi(a|\itup{s,u}) \\
- r(s, \bi u{\alpha+\beta}) \\
- \gamma \E_{s' \sim \mathcal{D}}[ \\
\E_{\epsilon_{t+1} \sim \mathcal{N}}[ \\
- \log \pi(a_{t+1} \mid \itup{s',(a, \bisn u1{-1})}) \\
+ r(s', a_{t-\alpha-\beta+1}) \\
+\gamma \E_{s_{t-\alpha+2} \sim \mathcal{D}}[ \\
v(\itup{s_{t-\alpha+2},\slice{a}{t+1}{t-\alpha-\beta+2}})
]]]]
\end{multline}
%}

We rearrange this:
%{\small
\begin{multline}
\medmuskip=0mu
\thinmuskip=0mu
\thickmuskip=0mu
L^\text{SAC}_{\mathit{CDMDP}(E)}(\pi) = 
- \E_{\itup{s,u}, \sli{s}{t-\alpha+1}{t-\alpha+2} \sim \mathcal{D}} [\\
\sum_{i=t}^{t+1} \gamma^{i-t} r(s_{i-\alpha}, a_{i-\alpha-\beta}) \\
\E_{\sli{\epsilon}{t}{t+1} \sim \mathcal{N}}[ \\
- \sum_{i=t}^{t+1}
\gamma^{i-t} \log \pi(a_{i} \mid \itup{s_{i-\alpha},\slice{a}{i-1}{i-\alpha-\beta}}) \\
+ \gamma^2 v(\itup{s_{t-\alpha+2},\slice{a}{t+1}{t-\alpha-\beta+2}})
]]]
\end{multline}
%}




%%%%%%%%%%%%%%%%%%%%%%%%%%%%%%%%%%%%%%%%%%%ù PROOFS SAVE



\begin{proof}
The SAC algorithm maximizes an expected sum of discounted entropy-augmented rewards. The authors define a soft state-value function as:
$$
v^{\mathit{SAC}}_{\mathit{MDP}(E)}(s) =
\E_{a \sim \pi(\cdot \mid s)}[
q^{\mathit{SAC}}_{\mathit{MDP}(E)}(s, a) -
\log \pi (a \mid s)
]
$$

The SAC value iteration is the usual 1-step Bellman backup:
$$
% \mathcal{T}^\pi
q^{\mathit{SAC}}_{\mathit{MDP}(E)}(s, a) = r(s, a) +
\gamma \E_{s' \sim p(\cdot \mid s, a)}[
v^{\mathit{SAC}}_{\mathit{MDP}(E)}(s')
]
$$

The equivalents in the $\mathit{CDMDP}$ setting are:
\begin{equation}\medmuskip=0mu\thinmuskip=0mu\thickmuskip=0mu
\label{eq_soft_v_cd}
v (\itup{s,u}) =
\E_{a \sim \pi(\cdot \mid \itup{s,u})}[
q(\itup{s,u}, a) 
- \log \pi(a \mid \itup{s,u})
]
\end{equation}
And:
\begin{equation}
\medmuskip=0mu\thinmuskip=0mu\thickmuskip=0mu
\label{eq_soft_q_cd}
q(\itup{s,u}, a) = 
r(s, \bi u{\alpha+\beta})
+\gamma \E_{s' \sim p(\cdot \mid s, \bi u{\alpha+\beta})}[
v(\itup{s',(a, \bisn u1{-1})})
]
\end{equation}

Substituting \ref{eq_soft_q_cd} in \ref{eq_soft_v_cd} yields:
\begin{equation}
v (\itup{s,u}) = 
\E_{a \sim \pi(\cdot \mid \itup{s,u})}[
r(s, \bi u{\alpha+\beta})
+ \gamma \E_{s' \sim p(\cdot \mid s, \bi u{\alpha+\beta})}[
v(\itup{s',(a, \bisn u1{-1})})]
- \log \pi(a \mid \itup{s,u})
]
\end{equation}
Which can be rearranged as the result.

%Thus, the recursive definition of the soft value function in a $\mathit{CDMDP}$ is:

% <SIMON>
% \vspace{1cm}
% \noindent\rule{\textwidth}{0.5pt}
%
%\begin{definition}
%In a $\text{CDMDP}(E, \alpha, \beta)$ the entropy-augmented value function is:
%{\begin{equation}\medmuskip=0mu\thinmuskip=0mu\thickmuskip=0mu
%    v(\underbrace{\itup{s_{t-\alpha}, \ \sli a{t-\alpha-\beta}{t-1}}}_{x_t})
%    = r(s_{t-\alpha}, a_{t-\alpha-\beta})
%    + \mathbb{E}[\gamma v(\itup{s', \ \sli a {t-\alpha-\beta+1}{t}})
%    - \log \pi(a_t | \itup{s_{t-\alpha}, \ \sli a {t-\alpha-\beta}{t-1}})],
%\end{equation}}

%where $s' \sim p(\cdot|s_{t-\alpha}, a_{t-\alpha-\beta})$
%and $a_t \sim \pi(\cdot |\itup{s', \sli a {t-\alpha-\beta}{t-1}})$.
%\end{definition}
\end{proof}











%%%%%%%%%%%%%%%%%%%%%%%%%%%%%%%%%%%%%%%%%ù




\begin{proof}
\TODO{rewrite with this proof the new way of writing the result}
 \label{proof:actor-loss}
 
We have defined the DC/AC actor loss as:
\begin{equation}
L^{\textrm{DC/AC}}_\pi(\pi) = - \E_{x, \tau_{\alpha+\beta} \sim \mathcal D} [\hat v_{\alpha+\beta}^\text{soft}(x; \ \tau_{\alpha+\beta})]
\end{equation}

With:
\begin{multline}\small\medmuskip=0mu\thinmuskip=0mu\thickmuskip=0mu
    \hat v^\text{soft}_n(\itup{s_0, u}; \ \itup{s_1, u'}, x_2, ..., x_n)
    = \\
    r(s_0, \ \bi {u}{\alpha+\beta})
    + \E_{a\sim\pi(\cdot|\itup{s_0, u})}[
    \gamma v^\text{soft}_{n-1}(\itup{s_1, (a, \bisn{u}1{-1})}; \ x_2, ..., x_n)
    - \log \pi (a|\itup{s_0,u})]
\end{multline}
where $\hat v^\text{soft}_0$ is now unbiased.

To derive this formulation, we actually started from the SAC policy loss, which is defined in \cite{haarnoja2018soft} as:
\begin{equation}
    L^\text{SAC}_E(\pi) = \E_{s \sim \mathcal{D}} \KL(\pi(\cdot \mid s) \| \exp (q(s, \cdot)) / Z(s))
\end{equation}

Translated to the $\mathit{CDMDP}$ setting, this is:
\begin{equation}
    L^\text{SAC}_{\mathit{CDMDP}(E)}(\pi) = 
    \E_{\itup{s,u} \sim \mathcal{D}} [
    \KL\left( \pi \Big(\cdot \mid \itup{s,u}\Big) \bigg\|
    \frac{\exp (q \Big(\itup{s,u}, \cdot\Big))}{ Z(\itup{s,u})} \right) ]
\end{equation}
where the $\cdot$ random variable represents the action $a$ sampled from the current policy $\pi$.

Since we are ultimately interested in $\nabla_{\pi} L^\text{SAC}_{\mathit{CDMDP}(E)}(\pi)$, we can ignore the $Z$ partition, similarly to Haarnoja et al. \cite{haarnoja2018soft}, because it only depends on the action-value, and not on the parameters of the policy. Thus:
\begin{equation}
\label{eq_kl_1}
    L^\text{SAC}_{\mathit{CDMDP}(E)}(\pi) = 
    \E_{\itup{s,u} \sim \mathcal{D}} [
    \KL\left( \pi \Big(\cdot \mid \itup{s,u}\Big) \bigg\|
    \exp (q \Big(\itup{s,u}, \cdot\Big)) \right) ]
\end{equation}
We represent the policy by a neural network with an input noise vector $\epsilon \sim \mathcal{N}$ and can apply the reparameterization trick:
$$
a = \pi(x) = h_\pi(x, \epsilon)
$$

%To simplify notations, we denote $a_{i \geq t} := h_\pi (\itup{s_{i-\alpha},\slice{a}{i-1}{i-\alpha-\beta}}, \epsilon_i)$ and we do the derivation with sampled estimators directly.
Then:
%{\small
\begin{equation}
\medmuskip=0mu
\thinmuskip=0mu
\thickmuskip=0mu
L^\text{SAC}_{\mathit{CDMDP}(E)}(\pi) = 
\E_{\itup{s,u} \sim \mathcal{D}, \epsilon \sim \mathcal{N}} [\log\pi(a|\itup{s,u}) - q (\itup{s,u}, a)  ]
\end{equation}
%}

And since:
\begin{equation}
q(\itup{s,u}, ) =
r(s, \bi u{\alpha+\beta})
+\gamma \E_{s' \sim \mathcal{D}}[
v(\itup{s',(a, \bisn u1{-1})})
]
\end{equation}

We can further extend this loss as:
%{\small
\begin{equation}
\medmuskip=0mu
\thinmuskip=0mu
\thickmuskip=0mu
L^\text{SAC}_{\mathit{CDMDP}(E)}(\pi) = 
\E_{\itup{s,u} \sim \mathcal{D}, \epsilon \sim \mathcal{N}} [
\log\pi(a|\itup{s,u}) 
- r(s, \bi u{\alpha+\beta}) 
- \gamma \E_{s' \sim \mathcal{D}}[ 
v (\itup{s',(a, \bisn u1{-1})})]
\end{equation}
%}

$r(s, \bi u{\alpha+\beta})$ can be moved out of the expectation over $\mathcal{N}$ as it does not depend on $a$:
%{\small
\begin{equation}
\medmuskip=0mu
\thinmuskip=0mu
\thickmuskip=0mu
L^\text{SAC}_{\mathit{CDMDP}(E)}(\pi) = 
-
\E_{\itup{s,u}, s' \sim \mathcal{D}} [
r(s, \bi u{\alpha+\beta})
+
\E_{\epsilon \sim \mathcal{N}} [
\gamma 
v (\itup{s',(a, \bisn u1{-1})})
- \log\pi(a|\itup{s,u})
]]
\end{equation}
%}

If $v^\text{soft}_0$ is unbiased, this directly maps to the soft state-value estimator ???



And unrolling this equation for the whole $\tau_{\alpha+\beta}$ trajectory sampled in $\mathcal{D}$ we get:

%{\small
\begin{multline}
\medmuskip=0mu
\thinmuskip=0mu
\thickmuskip=0mu
L^\text{SAC}_{\mathit{CDMDP}(E)}(\pi) = \\ 
- \E_{\itup{s,u}, \sli{s}{t-\alpha+1}{t+\beta} \sim \mathcal{D}} [\\
\sum_{i=t}^{t+\alpha+\beta-1} \gamma^{i-t} r(s_{i-\alpha}, a_{i-\alpha-\beta}) \\
+ \E_{\sli{\epsilon}{t}{t+\alpha+\beta-1} \sim \mathcal{N}} [ \\
- \sum_{i=t}^{t+\alpha+\beta-1}
\gamma^{i-t} \log \pi(a_{i} \mid \itup{s_{i-\alpha},\slice{a}{i-1}{i-\alpha-\beta}}) \\
+ \gamma^{\alpha+\beta} v(\itup{s_{t+\beta},\slice{a}{t+\alpha+\beta-1}{t}})
]]
\end{multline}
%}
where the $a_{i \geq t} := h_\pi (\itup{s_{i-\alpha},\slice{a}{i-1}{i-\alpha-\beta}}, \epsilon_i)$ are unrolled.

Note that the first sum does not depend on the parameters of $\pi$ because $u$ and $\sli{s}{t-\alpha}{t+\beta-1}$ are sampled from $\mathcal{D}$. Therefore we can define the following gradient-equivalent loss:
%{\small
\begin{multline}
\medmuskip=0mu
\thinmuskip=0mu
\thickmuskip=0mu
L^\textrm{DC/AC}(\pi) = (\dots) = \\ 
- \E_{\itup{s,u}, \sli{s}{t-\alpha+1}{t+\beta} \sim \mathcal{D}, \sli{\epsilon}{t}{t+\alpha+\beta-1} \sim \mathcal{N}} [\\
- \sum_{i=t}^{t+\alpha+\beta-1}
\gamma^{i-t} \log \pi(a_{i} \mid \itup{s_{i-\alpha},\slice{a}{i-1}{i-\alpha-\beta}}) \\
+ \gamma^{\alpha+\beta} v(\itup{s_{t+\beta},\slice{a}{t+\alpha+\beta-1}{t}})
]
\end{multline}
%}
where the $a_{i \geq t} := h_\pi (\itup{s_{i-\alpha},\slice{a}{i-1}{i-\alpha-\beta}}, \epsilon_i)$ are unrolled.
\end{proof}



%%%%%%%%%%%%%%%%%%%%%%%%%%%%%%%%%%%


And since:
\begin{equation}
q(\itup{s,u}, ) =
r(s, \bi u{\alpha+\beta})
+\gamma \E_{s' \sim \mathcal{D}}[
v(\itup{s',(a, \bisn u1{-1})})
]
\end{equation}

We can further extend this loss as:
%{\small
\begin{equation}
\medmuskip=0mu
\thinmuskip=0mu
\thickmuskip=0mu
L^\text{SAC}_{\mathit{CDMDP}(E)}(\pi) = 
\E_{\itup{s,u} \sim \mathcal{D}, \epsilon \sim \mathcal{N}} [
\log\pi(a|\itup{s,u}) 
- r(s, \bi u{\alpha+\beta}) 
- \gamma \E_{s' \sim \mathcal{D}}[ 
v (\itup{s',(a, \bisn u1{-1})})]
\end{equation}
%}

$r(s, \bi u{\alpha+\beta})$ can be moved out of the expectation over $\mathcal{N}$ as it does not depend on $a$:
%{\small
\begin{equation}
\medmuskip=0mu
\thinmuskip=0mu
\thickmuskip=0mu
L^\text{SAC}_{\mathit{CDMDP}(E)}(\pi) = 
-
\E_{\itup{s,u}, s' \sim \mathcal{D}} [
r(s, \bi u{\alpha+\beta})
+
\E_{\epsilon \sim \mathcal{N}} [
\gamma 
v (\itup{s',(a, \bisn u1{-1})})
- \log\pi(a|\itup{s,u})
]]
\end{equation}
%}

If $v^\text{soft}_0$ is unbiased, this directly maps to the soft state-value estimator ???



And unrolling this equation for the whole $\tau_{\alpha+\beta}$ trajectory sampled in $\mathcal{D}$ we get:

%{\small
\begin{multline}
\medmuskip=0mu
\thinmuskip=0mu
\thickmuskip=0mu
L^\text{SAC}_{\mathit{CDMDP}(E)}(\pi) = \\ 
- \E_{\itup{s,u}, \sli{s}{t-\alpha+1}{t+\beta} \sim \mathcal{D}} [\\
\sum_{i=t}^{t+\alpha+\beta-1} \gamma^{i-t} r(s_{i-\alpha}, a_{i-\alpha-\beta}) \\
+ \E_{\sli{\epsilon}{t}{t+\alpha+\beta-1} \sim \mathcal{N}} [ \\
- \sum_{i=t}^{t+\alpha+\beta-1}
\gamma^{i-t} \log \pi(a_{i} \mid \itup{s_{i-\alpha},\slice{a}{i-1}{i-\alpha-\beta}}) \\
+ \gamma^{\alpha+\beta} v(\itup{s_{t+\beta},\slice{a}{t+\alpha+\beta-1}{t}})
]]
\end{multline}
%}
where the $a_{i \geq t} := h_\pi (\itup{s_{i-\alpha},\slice{a}{i-1}{i-\alpha-\beta}}, \epsilon_i)$ are unrolled.

Note that the first sum does not depend on the parameters of $\pi$ because $u$ and $\sli{s}{t-\alpha}{t+\beta-1}$ are sampled from $\mathcal{D}$. Therefore we can define the following gradient-equivalent loss:
%{\small
\begin{multline}
\medmuskip=0mu
\thinmuskip=0mu
\thickmuskip=0mu
L^\textrm{DC/AC}(\pi) = (\dots) = \\ 
- \E_{\itup{s,u}, \sli{s}{t-\alpha+1}{t+\beta} \sim \mathcal{D}, \sli{\epsilon}{t}{t+\alpha+\beta-1} \sim \mathcal{N}} [\\
- \sum_{i=t}^{t+\alpha+\beta-1}
\gamma^{i-t} \log \pi(a_{i} \mid \itup{s_{i-\alpha},\slice{a}{i-1}{i-\alpha-\beta}}) \\
+ \gamma^{\alpha+\beta} v(\itup{s_{t+\beta},\slice{a}{t+\alpha+\beta-1}{t}})
]
\end{multline}
%}
where the $a_{i \geq t} := h_\pi (\itup{s_{i-\alpha},\slice{a}{i-1}{i-\alpha-\beta}}, \epsilon_i)$ are unrolled.
